# Supplementary material for: Gaze-Contingent Ocular Parallax Rendering for Virtual Reality
Source: arXiv:1906.09740 source file (2020-05-13)
Supplement: Supplementary file 1 [file supplement_disparity.tex]

% !TeX root = ../supplement.tex

In Figure~\ref{fig:supp:disparity}, we show additional details for calculating the disparity distortions of objects in the periphery of the visual field. On the right, we illustrate the settings we simulated: a user fixating on the optical axis on one of four different depths, either 1~D (1~m), 2~D (50~cm), 3~D (33.3~cm), or 4~D (25~cm). For each of these fixation distances, we then traced out points with the same respective distance from the center point between the eyes along an arc (red points). We then calculated what the disparity angles to left and right eye would be when rays go directly from the individual points through the center of rotation of the eyes and when they go through the front nodal point. The discrepancy between these disparity angles is plotted for all four distance settings and for a range of eccentricity angles (i.e., points moving along the arc) in the left. We see that the disparity distortion is zero for foveal vision, but steadily increases the farther we go into peripheral vision. Although the disparity distortion measured in angles of visual degrees is more pronounced for closer distances, when converting these distortion to meters, they are fairly independent of depth (center). However, the maximum depth distortion is only about 4~mm at an eccentricity of $60^{\circ}$, which is negligible. The perceived location of the distorted points is also rendered by blue dots on the right, showing that they are fairly close to the target points. 

While these distortions increase in the periphery, they may not be perceptible because stereoacuity also decreases in the periphery~\cite{Rawlings:69,McKee:83}. For example, stereoacuity at 10\textdegree\ eccentricity was measured to be 80~arcsec~\cite{Fendick:83}. In comparison, the expected amount of disparity distortion due to a lack of appropriate ocular parallax rendering at 10\textdegree\ eccentricity is 73.76 arcsec (fixating at 4~D). This implies that the disparity distortions of conventional stereo rendering in peripheral vision may be too small to have a measurable effect on depth perception, which was indeed verified by the egocentric distance estimation study in the main paper. However, the micro parallax and gaze-contingent occlusion induced by ocular parallax rendering were shown to improve ordinal depth estimation and create a stronger impression of realistic depth. 

\begin{figure}[h]
	\centering
		\includegraphics[width=\textwidth]{disparity_distortion_supplement.pdf}
		\caption{Simulated conditions for estimating disparity distortions caused by conventional stereo rendering (right). The amount of expected disparity distortion is expected to be zero for foveal vision and increasing in the periphery of the visual field (left). When converted to perceived depth distortion (center), the expected amount of distortion, even in the periphery, is negligible and perhaps imperceivable.}
		\label{fig:supp:disparity}
\end{figure}
