# Supplementary material for: Gaze-Contingent Ocular Parallax Rendering for Virtual Reality
Source: arXiv:1906.09740 source file (2020-05-13)
Supplement: Supplementary file 2 [file supplement_stereopreference.tex]

% !TeX root = ../supplement.tex

\begin{figure}[t]
	\centering
		\includegraphics[width=\columnwidth]{user_study/preference_study.pdf}
		\caption{Subjective depth perception. We asked users to rank conventional rendering, ocular parallax rendering, and reversed ocular parallax rendering by how effective these modes are in conveying the 3D structure of the scene. Neither the monocular nor the binocular conditions show a significant effect for any of the scenes (top row).}
		\label{fig:preference}
\end{figure}

In addition to measuring the effect of ocular parallax rendering on egocentric depth perception with the blind reaching task, we were also interested in evaluating depth perception in a more subjective way and studying if reversing the parallax direction would affect the experience. To this end, we designed a user experiment that allowed users to rank three different rendering modes in multiple conditions: conventional rendering, ocular parallax rendering, and reversed ocular parallax rendering. We studied the subjective user perception of these modes in monocular and stereoscopic viewing conditions with three scenes each. These scenes show a city scene from near, middle, and far viewpoints with the distance between background and closest foreground object being 3~D, 2~D, and 1~D, respectively. For this study, we tested 16 users (age range, 22\textendash29, 5 female), of which one was excluded for not passing a standard Randot stereo vision test, and two others were excluded due to the eye tracker failing to track their pupils. For each scene viewpoint (\autoref{fig:preference}, top), users were shown each rendering mode for 20 seconds, after which they could switch between and rank the modes at will. The presentation order of the viewpoints and modes was randomized. Seven subjects started in the monocular condition, while six started in the binocular condition. Participants were encouraged to gaze around the scene liberally, although this instruction was not strictly enforced. Head pose tracking was disabled. Participants were asked to rank the three rendering modes based on how effective they were in conveying the 3D structure of the scene.

Results of the rankings are shown in \autoref{fig:preference}. On average, participants did not seem to think any particular mode conveyed the 3D structure of the scene better than others. A Friedman test was used to test for statistical significance, and no effect was found. Interestingly, almost all participants reported to have seen the effect during a post-study debriefing stating that they could see a change in perspective or viewing angle in the two ocular parallax modes. Many commented on observing noticeable latency (i.e., ``snapping'') in both ocular parallax modes, resulting in a reduced sense of immersion. The display and the eye tracking were verified to update correctly at 90~Hz and 120~Hz, respectively, resulting in a theoretical latency of about 20~ms. Note that this latency represents the state of the art of eye tracking technology available for head-mounted displays today. Given that our sensitivity to differential velocities is smaller than our minimum angle of resolution across the visual field~\cite{Mckee:84}, it seems as though significantly lower latency is required to fully remove noticeable jitter and delay between eye rotation and ocular parallax rendering.
